# Supplementary material for: RepoHyper: Search-Expand-Refine on Semantic Graphs for Repository-Level Code Completion
Source: arXiv:2403.06095 source file (2024-08-14)
Supplement: Supplementary file 1 [file sample_repohyper_appendix.pdf]

scapy/layers/smb2.py

```
# ... (imports omitted for brevity)
from scapy.fields import ByteField
from scapy.layers.gssapi import GSSAPI_BLOB
```

```
class SMB2_Error_Response(_SMB2_Payload):
    Command = -1
    __slots__ = ["NTStatus"] # extra info
    name = "SMB2 Error Response"
    fields_desc = [
        XLEShortField("StructureSize", 0x09),
        ByteField("ErrorContextCount", 0),
```

Current In-file  
Context

Direct similar search

```
class GSSAPI_BLOB(ASN1_Packet):
    ASN1_codec = ASN1_Codecs.BER
    ASN1_root = ASN1F_GSSAPI_APPLICATION(
        ASN1F_OID("MechType", "1.3.6.1.5.5.2"),
        ASN1F_PACKET(
            "innerToken",
            None,
            None,
            next_cls_cb=lambda pkt:
                _GSSAPI_OIDS.get(pkt.MechType.val, conf.raw_layer)))
```

Similar-based

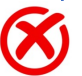

scapy/layers/smb2.py

```
class _SMB2_Payload(Packet):
    ...
```

```
class SMB2_Read_Request(_SMB2_Payload, _NTLMPayloadPacket):
    ...
    fields_desc = [
        XLEShortField("StructureSize", 0x31),
        ByteField("Padding", 0x00),
```

```
class ByteField(Field[int, int]):
    def __init__(self, name, default):
    ...
```

RepoHyper

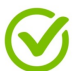

Search

Expand and Link

## Inversion\_bert.py

```
# ... (imports omitted for brevity)
from utils.sent_utils import get_similarity_metric
from invert.models import MultiLabelInversionModel,
MultiSetInversionModel

def optimization_inversion():
    ...
    if FLAGS.low_layer_idx == 0:
        encoded = mean_pool(...)
    else:
        encoded = encode(...)
    targets = ...
    loss = get_similarity_metric(encoded, targets,
                                FLAGS.metric, rtn_loss=True)
```

Current In-file  
Context

Direct similar search

```
class MultiLabelInversionModel(object):
    def __init__(...):
        ...
        if init_word_emb is not None:
            self.embedding = ...
        else:
            self.embedding = None
```

Similar-based

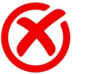

## Inversion\_albert.py

```
def optimization_inversion():
    ...
    if FLAGS.low_layer_idx == 0:
        ...
    else:
        ...
    loss = get_similarity_metric

def get_similarity_metric(x, y, metric, rtn_loss=False):
    if metric == 'cosine':
        x = tf.nn.l2_normalize(x, axis=-1)
    ...
```

RepoHyper

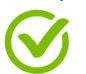

Search

Expand and Link





```

# ... (many imports omitted for brevity)
> from utils.utils import write_to_csv, get_csv_writer, \ ...

class _Statemachine(object):
    #... (methods omitted for brevity)
    def _csv_hash_running_process(self, list_running):
        with open(self.output_dir + '%s_hash_processes' % \
            self.computer_name + self.rand_ext, 'ab') as fw:
            csv_writer = get_csv_writer(fw)
            write_to_csv(["COMPUTER_NAME", "TYPE", "PID", "PROCESS_NAME",
                "SHA1", "CTIME", "MTIME", "ATIME"], csv_writer,
                self.output_dir + self.computer_name + '_sha256.log')
    #... (methods omitted for brevity)
    def _csv_list_running_process(self, list_running):
        with open(self.output_dir + '%s_processes' % self.computer_name + \
            self.rand_ext, 'ab') as fw:
            csv_writer = get_csv_writer(fw)
            write_to_csv(
                ["COMPUTER_NAME", "TYPE", "PID", \
                "PROCESS_NAME", "COMMAND", "EXEC_PATH"], csv_writer
            )

```

```

def write_to_csv(arr_data, csv_writer):\r\n
    """Writes contents to a CSV file using UTF-8"""
    csv_writer.writerow(arr_data)

```

RSG-based

```

def get_csv_writer(csvfile):
    return UnicodeWriter(csvfile, quoting=csv.QUOTE_ALL)

```

Similar-based
